# Supplementary material for: PointLLM: Empowering Large Language Models to Understand Point Clouds
Source: arXiv:2308.16911 source file (2024-09-06)
Supplement: Supplementary file 18 [file instruction_lists_minipage.tex]

% \begin{table*}
% \begin{minipage}[h]{0.49\linewidth}
\newpage
\begin{table}
\caption{\textbf{The instruction list for brief descriptions.} An instruction from the list is randomly selected and coupled with a human-written caption from Cap3D\cite{Cap3D} to form a brief-description instruction following sample.}
% \vbox to 0.7\textheight{ % Adjust this height as needed
\scalebox{0.98}{\tablestyle{8pt}{1.0}
\label{tab:brief_des_prompt}
\begin{tabular}{@{}p{\linewidth}@{}} % Adjust the width as needed
\toprule
\begin{itemize}
\item Summarize the 3D point cloud object briefly.
\item What kind of object is depicted by this point cloud?
\item Provide a short explanation of this 3D structure.
\item What does this collection of points represent?
\item Offer a succinct summary of this 3D object.
\item Can you give a brief overview of this point cloud?
\item Characterize the object this point cloud is illustrating.
\item Share a brief interpretation of this 3D point cloud.
\item Provide an outline of this 3D shape's characteristics.
\item What object is this point cloud rendering?
\item Deliver a quick description of the object represented here.
\item How would you describe the 3D form shown in this point cloud?
\item What is the nature of the object this point cloud is representing?
\item Present a compact account of this 3D object's key features.
\item What can you infer about the object from this point cloud?
\item Offer a clear and concise description of this point cloud object.
\item How would you summarize this 3D data set?
\item Give a brief explanation of the object that this cloud of points forms.
\item What kind of structure does this 3D point cloud depict?
\item Could you delineate the form indicated by this point cloud?
\item Express in brief, what this point cloud is representing.
\item Give a quick overview of the object represented by this 3D cloud.
\item Convey a summary of the 3D structure represented in this point cloud.
\item What kind of object is illustrated by this collection of points?
\item Describe the object that this point cloud forms.
\item How would you interpret this 3D point cloud?
\item Can you briefly outline the shape represented by these points?
\item Give a concise interpretation of the 3D data presented here.
\item Explain the object this point cloud depicts succinctly.
\item Offer a summary of the 3D object illustrated by this cloud.
\end{itemize} \\ \bottomrule
\end{tabular}
}
% }
\end{table}
% \end{minipage}
% \hfill % Add horizontal space between the minipages
% \begin{minipage}[h]{0.49\linewidth}
\begin{table}
\caption{\textbf{The instruction list for detailed descriptions.} An instruction from the list is randomly selected and coupled with a GPT-4 generated caption to form a detailed-description instruction following sample.}
\label{tab:detailed_des_prompt}
% \vbox to 0.734\textheight{ % Adjust this height as needed
\scalebox{0.98}{\tablestyle{8pt}{1.0}
\begin{tabular}{@{}p{\linewidth}@{}} % Adjust the width as needed
\toprule
\begin{itemize}
\item Can you tell me more about this?
\item What does this represent?
\item Can you describe this in more detail?
\item I'm interested in this, can you explain?
\item What is this object made of?
\item Could you provide more info about this?
\item What exactly am I looking at here?
\item What is this?
\item Could you describe the detailed structure of this?
\item This looks interesting, can you expand on it?
\item Can you explain more about this form?
\item What can you tell me about the shape of this object?
\item Could you delve deeper into this?
\item I want to know more about this, can you help?
\item Can you walk me through the details of this object?
\item Can you provide a comprehensive account of this object?
\item Offer a detailed interpretation of this point cloud.
\item Please elucidate on the characteristics of this form.
\item Could you provide an in-depth description of this structure?
\item What does this cloud represent in its entirety?
\item Elaborate on the details of this point cloud, please.
\item Kindly furnish me with more information about this object.
\item Please expand on the intricate structure of this form.
\item Provide a meticulous explanation of what these points represent.
\item I request a detailed breakdown of this structure.
\item Give a thorough rundown of this point cloud.
\item Can you offer a complete analysis of this object?
\item I would like a comprehensive explanation of this form.
\item Please detail the specific features of this point cloud.
\item Could you elaborate extensively on what this represents?
\end{itemize} \\ \bottomrule
\end{tabular}
}
% }
\end{table}
% \end{minipage}
% \end{table*}
\clearpage
